# Supplementary material for: Vertex-reinforced Random Walk for Network Embedding
Source: arXiv:2002.04497 source file (2020-02-11)
Supplement: Supplementary file 1 [file appendix.tex]

% Please add the following required packages to your document preamble:
\usepackage{multirow}
\begin{table}[]
\begin{tabular}{cccccccccccc}
 &  & \multicolumn{5}{c}{Micro-F1} & \multicolumn{5}{c}{Macro-F1} \\
 &  & 0.1 & 0.3 & 0.5 & 0.7 & 0.9 & 0.1 & 0.3 & 0.5 & 0.7 & 0.9 \\
VRRW & w/o exploration & 8.6 & 9.8 & 10.9 & 11.7 & 12.7 & 5.3 & 8.1 & 8.9 & 9.6 & 10.0 \\
 & Greedy & 13.6 & 16.8 & 19.0 & 20.8 & 22.6 & 11.1 & 14.4 & 16.2 & 17.7 & 18.6 \\
 & UCB & 13.4 & 16.7 & 18.9 & 20.1 & 21.0 & 11.2 & 14.4 & 16.3 & 17.2 & 17.6 \\
\multirow{3}{*}{DRRW-KL} & w/o exploration & 8.5 & 10.0 & 10.9 & 11.7 & 13.1 & 6.7 & 8.5 & 9.3 & 9.8 & 10.6 \\
 & Greedy &  &  &  &  &  &  &  &  &  &  \\
 & UCB & 15.1 & 19.0 & 22.0 & 23.2 & 24.2 & 12.4 & 16.3 & 18.2 & 19.3 & 19.5 \\
\multirow{3}{*}{DRRW-JS} & w/o exploration & 8.3 & 9.6 & 10.7 & 11.2 & 12.3 & 6.5 & 7.9 & 9.1 & 9.3 & 9.6 \\
 & Greedy & 14.3 & 17.8 & 19.9 & 21.2 & 22.7 & 12.1 & 15.7 & 16.3 & 17.4 & 18.1 \\
 & UCB & 15.9 & 20.5 & 22.5 & 23.5 & 24.4 & 12.9 & 17.0 & 18.7 & 19.2 & 19.9
\end{tabular}
\end{table}
